# Supplementary material for: MolmoAct2: Action Reasoning Models for Real-world Deployment
Source: arXiv:2605.02881 source file (2026-05-08)
Supplement: Supplementary file 1 [file 5-data-examples.tex]

\section{Data Examples}
\label{supp:dataexamples}

This section include \textbf{randomly selected} examples from \molmoact's Action Reasoning Data and Multimodal web data used in pre-training, as well as \molmoactdata used in mid-training, and demonstrations collected for post-training. Prompts are shown in bold and Visual Reasoning Trace are annotated with a yellow line.

\begin{itemize}
    \item \textbf{Action Reasoning Data - Figure \ref{fig:appendix_action_reasoning_data_1}}
    \item \textbf{Auxiliary Visual Reasoning Trace - Figure \ref{fig:appendix_line} }
    \item \textbf{Auxiliary Depth Perception Tokens - Figure \ref{fig:appendix_depth}}
    \item \textbf{Trajectory-conditioned Action Data - Figure \ref{fig:appendix_trajectory}}
    \item \textbf{Multimodal Web Data - Figure \ref{fig:appendix_vqa}}
    \item \textbf{\molmoactdata (Home Environment) - Figure \ref{fig:appendix_molmoactdataset_home}}
    \item \textbf{\molmoactdata (Tabletop) - Figure \ref{fig:appendix_molmoactdataset_tabletop}}
    \item \textbf{Post-Training Single Arm Franka - Figure \ref{fig:appendix_singlearm}}
    \item \textbf{Post-Training Bimanual Franka - Figure \ref{fig:appendix_bimanual}}
    \item \textbf{Post-Training Rainbow - Figure \ref{fig:appendix_rainbow}}
    
\end{itemize}

\begin{figure*}[t]  
  \centering
  \includegraphics[width=\textwidth]{figures/Appendix/Data_Examples/Appendix_Action_Reasoning_1.pdf}
  \caption{Randomly selected examples from \textbf{Action Reasoning Data} used in the pre-training stage.}

  \label{fig:appendix_action_reasoning_data_1}
\end{figure*}

\begin{figure*}[t]  
  \centering
  \includegraphics[width=\textwidth]{figures/Appendix/Data_Examples/Appendix_Line_2.pdf}
  \caption{Randomly selected examples from \textbf{Auxiliary Visual Reasoning Trace} data used in the pre-training stage.}

  \label{fig:appendix_line}
\end{figure*}

\begin{figure*}[t]  
  \centering
  \includegraphics[width=\textwidth]{figures/Appendix/Data_Examples/Appendix_Depth_2.pdf}
  \caption{Randomly selected examples from \textbf{Auxiliary Depth Perception Tokens} data used in the pre-training stage.}

  \label{fig:appendix_depth}
\end{figure*}

\begin{figure*}[t]  
  \centering
  \includegraphics[width=\textwidth]{figures/Appendix/Data_Examples/Appendix_Trajectory.pdf}
  \caption{Randomly selected examples from \textbf{Trajectory-conditioned Action Data} used in the pre-training stage.}

  \label{fig:appendix_trajectory}
\end{figure*}

\begin{figure*}[t]  
  \centering
  \includegraphics[width=\textwidth]{figures/Appendix/Data_Examples/Appendix_VQA.pdf}
  \caption{Randomly selected examples from \textbf{Multimodal Web Data} used in the pre-training stage.}

  \label{fig:appendix_vqa}
\end{figure*}

\begin{figure*}[t]  
  \centering
  \includegraphics[width=\textwidth]{figures/Appendix/Data_Examples/Appendix_Molmoact_Home.pdf}
  \caption{Randomly selected examples from \textbf{\molmoactdata (Home Environment)} used in the mid-training stage.}

  \label{fig:appendix_molmoactdataset_home}
\end{figure*}

\begin{figure*}[t]  
  \centering
  \includegraphics[width=\textwidth]{figures/Appendix/Data_Examples/Appendix_Molmoact_Tabletop.pdf}
  \caption{Randomly selected examples from \textbf{\molmoactdata (Tabletop Environment)} used in the mid-training stage.}

  \label{fig:appendix_molmoactdataset_tabletop}
\end{figure*}

\begin{figure*}[t]  
  \centering
  \includegraphics[width=\textwidth]{figures/Appendix/Data_Examples/Appendix_SingleArm.pdf}
  \caption{Randomly selected examples from \textbf{Single Arm Franka} demonstrations used in the post-training stage.}

  \label{fig:appendix_singlearm}
\end{figure*}

\begin{figure*}[t]  
  \centering
  \includegraphics[width=\textwidth]{figures/Appendix/Data_Examples/Appendix_Bimanual.pdf}
  \caption{Randomly selected examples from \textbf{Bimanual Franka} demonstrations used in the post-training stage.}

  \label{fig:appendix_bimanual}
\end{figure*}

\begin{figure*}[t]  
  \centering
  \includegraphics[width=\textwidth]{figures/Appendix/Data_Examples/Appendix_Rainbow.pdf}
  \caption{Randomly selected examples from \textbf{Rainbow} demonstrations used in the post-training stage.}

  \label{fig:appendix_rainbow}
\end{figure*}
