# Supplementary material for: MolmoAct2: Action Reasoning Models for Real-world Deployment
Source: arXiv:2605.02881 source file (2026-05-08)
Supplement: Supplementary file 2 [file action_vocab_1.tex]

% NOTE: Compile with XeLaTeX or LuaLaTeX to render UTF-8 token glyphs.
\begin{table*}[!htbp]
\centering
\footnotesize
\setlength{\tabcolsep}{1pt}
\setlength{\arrayrulewidth}{0.1pt}

\caption{\textbf{Action token vocabulary}: Mapping from discrete bin index (0 to 127) to the actual token string.}
\label{tab:action_vocab_1}
\begin{tabular}{r l r l r l r l}
\toprule
\textbf{Bin} & \textbf{| Action Token} & \textbf{Bin} & \textbf{| Action Token} & \textbf{Bin} & \textbf{| Action Token} & \textbf{Bin} & \textbf{| Action Token} \\
\midrule
0 & \texttt{\textbackslash{}u00e2\textbackslash{}u00bd\textbackslash{}u0139} & 1 & \texttt{\textbackslash{}u00e2\textbackslash{}u00ba\textbackslash{}u0141} & 2 & \texttt{\textbackslash{}u00e2\textbackslash{}u012f\textbackslash{}u00a8} & 3 & \texttt{\textbackslash{}u00e1\textbackslash{}u0137\textbackslash{}u00b7} \\
4 & \texttt{\textbackslash{}u00ef\textbackslash{}u00a8\textbackslash{}u012c} & 5 & \texttt{\textbackslash{}u00e3\textbackslash{}u0129\textbackslash{}u00bd} & 6 & \texttt{\textbackslash{}u00e3\textbackslash{}u0129\textbackslash{}u00ba} & 7 & \texttt{\textbackslash{}u00e2\textbackslash{}u00bd\textbackslash{}u00ba} \\
8 & \texttt{\textbackslash{}u00e2\textbackslash{}u0134\textbackslash{}u0142} & 9 & \texttt{\textbackslash{}u00e3\textbackslash{}u012c\textbackslash{}u00a5} & 10 & \texttt{\textbackslash{}u00e2\textbackslash{}u00bc\textbackslash{}u0143} & 11 & \texttt{\textbackslash{}u00e2\textbackslash{}u00b0\textbackslash{}u00a1} \\
12 & \texttt{\textbackslash{}u00e2\textbackslash{}u00b0\textbackslash{}u0142} & 13 & \texttt{\textbackslash{}u00e2\textbackslash{}u00b0\textbackslash{}u0141} & 14 & \texttt{\textbackslash{}u00e2\textbackslash{}u00b0\textbackslash{}u0133} & 15 & \texttt{\textbackslash{}u00e2\textbackslash{}u00b0\textbackslash{}u0132} \\
16 & \texttt{\textbackslash{}u00e2\textbackslash{}u00b0\textbackslash{}u0130} & 17 & \texttt{\textbackslash{}u00e2\textbackslash{}u00b0\textbackslash{}u012f} & 18 & \texttt{\textbackslash{}u00e2\textbackslash{}u00b0\textbackslash{}u0124} & 19 & \texttt{\textbackslash{}u00e2\textbackslash{}u0134\textbackslash{}u00a1} \\
20 & \texttt{\textbackslash{}u00e2\textbackslash{}u0134\textbackslash{}u0141} & 21 & \texttt{\textbackslash{}u00e2\textbackslash{}u0122\textbackslash{}u00b4} & 22 & \texttt{\textbackslash{}u00e2\textbackslash{}u0136\textbackslash{}u00b2} & 23 & \texttt{\textbackslash{}u00f0\textbackslash{}u0135\textbackslash{}u0131\textbackslash{}u00a7} \\
24 & \texttt{\textbackslash{}u00ef\textbackslash{}u00a8\textbackslash{}u00b7} & 25 & \texttt{\textbackslash{}u00e3\textbackslash{}u012a\textbackslash{}u00bc} & 26 & \texttt{\textbackslash{}u00e2\textbackslash{}u0140\textbackslash{}u00b6} & 27 & \texttt{\textbackslash{}u00e2\textbackslash{}u0138\textbackslash{}u00a4} \\
28 & \texttt{\textbackslash{}u00e2\textbackslash{}u0129\textbackslash{}u0140} & 29 & \texttt{\textbackslash{}u00e2\textbackslash{}u0128\textbackslash{}u00b7} & 30 & \texttt{\textbackslash{}u00e2\textbackslash{}u0128\textbackslash{}u00a4} & 31 & \texttt{\textbackslash{}u00e1\textbackslash{}u00a5\textbackslash{}u00a4} \\
32 & \texttt{\textbackslash{}u00e1\textbackslash{}u00a5\textbackslash{}u0136} & 33 & \texttt{\textbackslash{}u00e1\textbackslash{}u0127\textbackslash{}u00a3} & 34 & \texttt{\textbackslash{}u00e0\textbackslash{}u00ba\textbackslash{}u0124} & 35 & \texttt{\textbackslash{}u00ef\textbackslash{}u00b1\textbackslash{}u012c} \\
36 & \texttt{\textbackslash{}u00ea\textbackslash{}u00a6\textbackslash{}u0136} & 37 & \texttt{\textbackslash{}u00e3\textbackslash{}u012b\textbackslash{}u00ab} & 38 & \texttt{\textbackslash{}u00e3\textbackslash{}u0127\textbackslash{}u0138} & 39 & \texttt{\textbackslash{}u00e3\textbackslash{}u0126\textbackslash{}u00a7} \\
40 & \texttt{\textbackslash{}u00e3\textbackslash{}u0126\textbackslash{}u0135} & 41 & \texttt{\textbackslash{}u00e3\textbackslash{}u0126\textbackslash{}u012f} & 42 & \texttt{\textbackslash{}u00e2\textbackslash{}u0141\textbackslash{}u00b0} & 43 & \texttt{\textbackslash{}u00e2\textbackslash{}u013f\textbackslash{}u00ab} \\
44 & \texttt{\textbackslash{}u00e2\textbackslash{}u013f\textbackslash{}u00aa} & 45 & \texttt{\textbackslash{}u00e2\textbackslash{}u013d\textbackslash{}u0131} & 46 & \texttt{\textbackslash{}u00e2\textbackslash{}u013d\textbackslash{}u0129} & 47 & \texttt{\textbackslash{}u00e2\textbackslash{}u0137\textbackslash{}u012c} \\
48 & \texttt{\textbackslash{}u00e2\textbackslash{}u0136\textbackslash{}u00bd} & 49 & \texttt{\textbackslash{}u00e1\textbackslash{}u00b8\textbackslash{}u012c} & 50 & \texttt{\textbackslash{}u00e1\textbackslash{}u00a4\textbackslash{}u012c} & 51 & \texttt{\textbackslash{}u00e1\textbackslash{}u013d\textbackslash{}u0132} \\
52 & \texttt{\textbackslash{}u00e1\textbackslash{}u013d\textbackslash{}u0127} & 53 & \texttt{\textbackslash{}u00e1\textbackslash{}u013c\textbackslash{}u012e} & 54 & \texttt{\textbackslash{}u00e1\textbackslash{}u013b\textbackslash{}u00b3} & 55 & \texttt{\textbackslash{}u00e0\textbackslash{}u0142\textbackslash{}u012e} \\
56 & \texttt{\textbackslash{}u00c6\textbackslash{}u012a} & 57 & \texttt{\textbackslash{}u00f0\textbackslash{}u0141\textbackslash{}u0127\textbackslash{}u0135} & 58 & \texttt{\textbackslash{}u00f0\textbackslash{}u0141\textbackslash{}u0127\textbackslash{}u0127} & 59 & \texttt{\textbackslash{}u00f0\textbackslash{}u013f\textbackslash{}u013c\textbackslash{}u0131} \\
60 & \texttt{\textbackslash{}u00f0\textbackslash{}u013f\textbackslash{}u013c\textbackslash{}u0126} & 61 & \texttt{\textbackslash{}u00f0\textbackslash{}u013f\textbackslash{}u013b\textbackslash{}u00bf} & 62 & \texttt{\textbackslash{}u00f0\textbackslash{}u013f\textbackslash{}u013b\textbackslash{}u00bd} & 63 & \texttt{\textbackslash{}u00f0\textbackslash{}u013f\textbackslash{}u013b\textbackslash{}u00bc} \\
64 & \texttt{\textbackslash{}u00f0\textbackslash{}u013f\textbackslash{}u013b\textbackslash{}u00ba} & 65 & \texttt{\textbackslash{}u00f0\textbackslash{}u013f\textbackslash{}u013b\textbackslash{}u00b8} & 66 & \texttt{\textbackslash{}u00f0\textbackslash{}u013f\textbackslash{}u013b\textbackslash{}u00b0} & 67 & \texttt{\textbackslash{}u00f0\textbackslash{}u013f\textbackslash{}u013b\textbackslash{}u00ae} \\
68 & \texttt{\textbackslash{}u00f0\textbackslash{}u013f\textbackslash{}u013a\textbackslash{}u013c} & 69 & \texttt{\textbackslash{}u00f0\textbackslash{}u013f\textbackslash{}u013a\textbackslash{}u0132} & 70 & \texttt{\textbackslash{}u00f0\textbackslash{}u013f\textbackslash{}u013a\textbackslash{}u0131} & 71 & \texttt{\textbackslash{}u00f0\textbackslash{}u013f\textbackslash{}u0138\textbackslash{}u0138} \\
72 & \texttt{\textbackslash{}u00f0\textbackslash{}u013f\textbackslash{}u0137\textbackslash{}u00b1} & 73 & \texttt{\textbackslash{}u00f0\textbackslash{}u013f\textbackslash{}u0137\textbackslash{}u00a1} & 74 & \texttt{\textbackslash{}u00f0\textbackslash{}u013f\textbackslash{}u0137\textbackslash{}u012f} & 75 & \texttt{\textbackslash{}u00f0\textbackslash{}u013f\textbackslash{}u0136\textbackslash{}u0135} \\
76 & \texttt{\textbackslash{}u00f0\textbackslash{}u013f\textbackslash{}u0135\textbackslash{}u00be} & 77 & \texttt{\textbackslash{}u00f0\textbackslash{}u013f\textbackslash{}u0135\textbackslash{}u00b9} & 78 & \texttt{\textbackslash{}u00f0\textbackslash{}u013f\textbackslash{}u0135\textbackslash{}u00ac} & 79 & \texttt{\textbackslash{}u00f0\textbackslash{}u013f\textbackslash{}u0135\textbackslash{}u0137} \\
80 & \texttt{\textbackslash{}u00f0\textbackslash{}u013f\textbackslash{}u0133\textbackslash{}u00b3} & 81 & \texttt{\textbackslash{}u00f0\textbackslash{}u0138\textbackslash{}u00a5\textbackslash{}u00a8} & 82 & \texttt{\textbackslash{}u00f0\textbackslash{}u0138\textbackslash{}u00a5} & 83 & \texttt{\textbackslash{}u00f0\textbackslash{}u0132\textbackslash{}u00b1\textbackslash{}u0127} \\
84 & \texttt{\textbackslash{}u00f0\textbackslash{}u0132\textbackslash{}u0143\textbackslash{}u012c} & 85 & \texttt{\textbackslash{}u00ef\textbackslash{}u0143\textbackslash{}u00b2} & 86 & \texttt{\textbackslash{}u00ef\textbackslash{}u00a5\textbackslash{}u00b1} & 87 & \texttt{\textbackslash{}u00ef\textbackslash{}u00a5\textbackslash{}u0142} \\
88 & \texttt{\textbackslash{}u00ef\textbackslash{}u00a4\textbackslash{}u00a6} & 89 & \texttt{\textbackslash{}u00ed\textbackslash{}u0135\textbackslash{}u00bb} & 90 & \texttt{\textbackslash{}u00ed\textbackslash{}u0135\textbackslash{}u00b6} & 91 & \texttt{\textbackslash{}u00ed\textbackslash{}u0135\textbackslash{}u00ae} \\
92 & \texttt{\textbackslash{}u00ed\textbackslash{}u0135\textbackslash{}u00ac} & 93 & \texttt{\textbackslash{}u00ed\textbackslash{}u012d\textbackslash{}u012f} & 94 & \texttt{\textbackslash{}u00ec\textbackslash{}u00bc\textbackslash{}u0129} & 95 & \texttt{\textbackslash{}u00ec\textbackslash{}u0128\textbackslash{}u012c} \\
96 & \texttt{\textbackslash{}u00eb\textbackslash{}u00a1\textbackslash{}u00bc} & 97 & \texttt{\textbackslash{}u00ea\textbackslash{}u00b3\textbackslash{}u0124} & 98 & \texttt{\textbackslash{}u00ea\textbackslash{}u00b2\textbackslash{}u00b4} & 99 & \texttt{\textbackslash{}u00ea\textbackslash{}u00b2\textbackslash{}u013b} \\
100 & \texttt{\textbackslash{}u00e4\textbackslash{}u00b6\textbackslash{}u00b5} & 101 & \texttt{\textbackslash{}u00e3\textbackslash{}u012a\textbackslash{}u00aa} & 102 & \texttt{\textbackslash{}u00e2\textbackslash{}u00b2\textbackslash{}u00a2} & 103 & \texttt{\textbackslash{}u00e2\textbackslash{}u013c\textbackslash{}u00a3} \\
104 & \texttt{\textbackslash{}u00e2\textbackslash{}u013a\textbackslash{}u00b5} & 105 & \texttt{\textbackslash{}u00e2\textbackslash{}u0136\textbackslash{}u0140} & 106 & \texttt{\textbackslash{}u00e1\textbackslash{}u00b8\textbackslash{}u00bb} & 107 & \texttt{\textbackslash{}u00e1\textbackslash{}u00b8\textbackslash{}u0125} \\
108 & \texttt{\textbackslash{}u00e1\textbackslash{}u00a8\textbackslash{}u0123} & 109 & \texttt{\textbackslash{}u00e1\textbackslash{}u0142\textbackslash{}u0126} & 110 & \texttt{\textbackslash{}u00e1\textbackslash{}u0136\textbackslash{}u012c} & 111 & \texttt{\textbackslash{}u00e1\textbackslash{}u0136\textbackslash{}u0127} \\
112 & \texttt{\textbackslash{}u00e1\textbackslash{}u0134\textbackslash{}u012e} & 113 & \texttt{\textbackslash{}u00e1\textbackslash{}u0132\textbackslash{}u00a7} & 114 & \texttt{\textbackslash{}u00e1\textbackslash{}u012e\textbackslash{}u0136} & 115 & \texttt{\textbackslash{}u00e1\textbackslash{}u012e\textbackslash{}u0126} \\
116 & \texttt{\textbackslash{}u00e1\textbackslash{}u012d\textbackslash{}u00a9} & 117 & \texttt{\textbackslash{}u00e1\textbackslash{}u012c\textbackslash{}u0134} & 118 & \texttt{\textbackslash{}u00e1\textbackslash{}u012b\textbackslash{}u00a8} & 119 & \texttt{\textbackslash{}u00e1\textbackslash{}u0123\textbackslash{}u00bc} \\
120 & \texttt{\textbackslash{}u00e1\textbackslash{}u0122\textbackslash{}u0131} & 121 & \texttt{\textbackslash{}u00e0\textbackslash{}u00b2\textbackslash{}u0141} & 122 & \texttt{\textbackslash{}u00e0\textbackslash{}u00b0\textbackslash{}u00b5} & 123 & \texttt{\textbackslash{}u00e0\textbackslash{}u00b0\textbackslash{}u00b3} \\
124 & \texttt{\textbackslash{}u00e0\textbackslash{}u00ac\textbackslash{}u012b} & 125 & \texttt{\textbackslash{}u00e0\textbackslash{}u00a5\textbackslash{}u00b1} & 126 & \texttt{\textbackslash{}u00e0\textbackslash{}u00a4\textbackslash{}u0133} & 127 & \texttt{\textbackslash{}u00dd\textbackslash{}u00a5} \\
\addlinespace[4pt]  
\bottomrule
\end{tabular}
\end{table*}
