# Supplementary material for: MolmoAct2: Action Reasoning Models for Real-world Deployment
Source: arXiv:2605.02881 source file (2026-05-08)
Supplement: Supplementary file 3 [file action_vocab_2.tex]

% NOTE: Compile with XeLaTeX or LuaLaTeX to render UTF-8 token glyphs.
\begin{table*}[!htbp]
\centering
\footnotesize
\setlength{\tabcolsep}{1pt}
\setlength{\arrayrulewidth}{0.1pt}

\caption{\textbf{Action token vocabulary}: Mapping from discrete bin index (128 to 255) to the actual token string.}
\label{tab:action_vocab_2}
\begin{tabular}{r l r l r l r l}
\toprule
\textbf{Bin} & \textbf{| Action Token} & \textbf{Bin} & \textbf{| Action Token} & \textbf{Bin} & \textbf{| Action Token} & \textbf{Bin} & \textbf{| Action Token} \\
\midrule
128 & \texttt{\textbackslash{}u00dd\textbackslash{}u0135} & 129 & \texttt{\textbackslash{}u00d4\textbackslash{}u0133} & 130 & \texttt{\textbackslash{}u00d4\textbackslash{}u012a} & 131 & \texttt{\textbackslash{}u00ca\textbackslash{}u00b6} \\
132 & \texttt{\textbackslash{}u00c8\textbackslash{}u00b2} & 133 & \texttt{\textbackslash{}u00f0\textbackslash{}u0141\textbackslash{}u0131\textbackslash{}u0129} & 134 & \texttt{\textbackslash{}u00f0\textbackslash{}u0141\textbackslash{}u0127\textbackslash{}u00a2} & 135 & \texttt{\textbackslash{}u00f0\textbackslash{}u013f\textbackslash{}u013c\textbackslash{}u0123} \\
136 & \texttt{\textbackslash{}u00f0\textbackslash{}u013f\textbackslash{}u013b\textbackslash{}u013e} & 137 & \texttt{\textbackslash{}u00f0\textbackslash{}u013f\textbackslash{}u0135\textbackslash{}u00b0} & 138 & \texttt{\textbackslash{}u00f0\textbackslash{}u013f\textbackslash{}u0135\textbackslash{}u0140} & 139 & \texttt{\textbackslash{}u00f0\textbackslash{}u0132\textbackslash{}u00b0\textbackslash{}u00bc} \\
140 & \texttt{\textbackslash{}u00f0\textbackslash{}u0132\textbackslash{}u0143\textbackslash{}u0135} & 141 & \texttt{\textbackslash{}u00f0\textbackslash{}u0132\textbackslash{}u00a4\textbackslash{}u0136} & 142 & \texttt{\textbackslash{}u00ef\textbackslash{}u00a8\textbackslash{}u0124} & 143 & \texttt{\textbackslash{}u00ef\textbackslash{}u00a7\textbackslash{}u00a9} \\
144 & \texttt{\textbackslash{}u00ef\textbackslash{}u00a6\textbackslash{}u0125} & 145 & \texttt{\textbackslash{}u00ef\textbackslash{}u00a4\textbackslash{}u0128} & 146 & \texttt{\textbackslash{}u00ef\textbackslash{}u00a4\textbackslash{}u0127} & 147 & \texttt{\textbackslash{}u00ed\textbackslash{}u013d\textbackslash{}u013e} \\
148 & \texttt{\textbackslash{}u00ed\textbackslash{}u0137\textbackslash{}u00b1} & 149 & \texttt{\textbackslash{}u00ed\textbackslash{}u0135\textbackslash{}u0143} & 150 & \texttt{\textbackslash{}u00ed\textbackslash{}u0135\textbackslash{}u0138} & 151 & \texttt{\textbackslash{}u00ed\textbackslash{}u0125\textbackslash{}u013b} \\
152 & \texttt{\textbackslash{}u00ed\textbackslash{}u0123\textbackslash{}u00bb} & 153 & \texttt{\textbackslash{}u00ec\textbackslash{}u00bb\textbackslash{}u0123} & 154 & \texttt{\textbackslash{}u00ec\textbackslash{}u00b3\textbackslash{}u0127} & 155 & \texttt{\textbackslash{}u00ec\textbackslash{}u013e\textbackslash{}u00be} \\
156 & \texttt{\textbackslash{}u00ec\textbackslash{}u013d\textbackslash{}u00a2} & 157 & \texttt{\textbackslash{}u00eb\textbackslash{}u00b1\textbackslash{}u0132} & 158 & \texttt{\textbackslash{}u00eb\textbackslash{}u00b1\textbackslash{}u012d} & 159 & \texttt{\textbackslash{}u00eb\textbackslash{}u00a7\textbackslash{}u0142} \\
160 & \texttt{\textbackslash{}u00eb\textbackslash{}u00a4\textbackslash{}u0124} & 161 & \texttt{\textbackslash{}u00eb\textbackslash{}u0138\textbackslash{}u00b0} & 162 & \texttt{\textbackslash{}u00e2\textbackslash{}u00a4\textbackslash{}u00a6} & 163 & \texttt{\textbackslash{}u00e2\textbackslash{}u00a1\textbackslash{}u00a2} \\
164 & \texttt{\textbackslash{}u00e2\textbackslash{}u013c\textbackslash{}u0139} & 165 & \texttt{\textbackslash{}u00e2\textbackslash{}u013c\textbackslash{}u0124} & 166 & \texttt{\textbackslash{}u00e2\textbackslash{}u013b\textbackslash{}u013b} & 167 & \texttt{\textbackslash{}u00e1\textbackslash{}u00bf\textbackslash{}u013c} \\
168 & \texttt{\textbackslash{}u00e1\textbackslash{}u00bf\textbackslash{}u0132} & 169 & \texttt{\textbackslash{}u00e1\textbackslash{}u00be\textbackslash{}u0136} & 170 & \texttt{\textbackslash{}u00e1\textbackslash{}u00b6\textbackslash{}u0131} & 171 & \texttt{\textbackslash{}u00e1\textbackslash{}u00a9\textbackslash{}u012d} \\
172 & \texttt{\textbackslash{}u00e1\textbackslash{}u00a8\textbackslash{}u00b8} & 173 & \texttt{\textbackslash{}u00e1\textbackslash{}u0142\textbackslash{}u00ac} & 174 & \texttt{\textbackslash{}u00e1\textbackslash{}u0142\textbackslash{}u0124} & 175 & \texttt{\textbackslash{}u00e1\textbackslash{}u0136\textbackslash{}u0143} \\
176 & \texttt{\textbackslash{}u00e1\textbackslash{}u012e\textbackslash{}u00bd} & 177 & \texttt{\textbackslash{}u00e1\textbackslash{}u012e\textbackslash{}u0125} & 178 & \texttt{\textbackslash{}u00e1\textbackslash{}u012b\textbackslash{}u0132} & 179 & \texttt{\textbackslash{}u00e1\textbackslash{}u012a\textbackslash{}u00be} \\
180 & \texttt{\textbackslash{}u00e1\textbackslash{}u012a\textbackslash{}u00a8} & 181 & \texttt{\textbackslash{}u00e1\textbackslash{}u012a\textbackslash{}u012c} & 182 & \texttt{\textbackslash{}u00e1\textbackslash{}u0128\textbackslash{}u00ba} & 183 & \texttt{\textbackslash{}u00e0\textbackslash{}u00bd\textbackslash{}u0127} \\
184 & \texttt{\textbackslash{}u00e0\textbackslash{}u00b4\textbackslash{}u00b4} & 185 & \texttt{\textbackslash{}u00d5\textbackslash{}u0125} & 186 & \texttt{\textbackslash{}u00ca\textbackslash{}u0135} & 187 & \texttt{\textbackslash{}u00c9\textbackslash{}u013a} \\
188 & \texttt{\textbackslash{}u00f0\textbackslash{}u0141\textbackslash{}u0137\textbackslash{}u012d} & 189 & \texttt{\textbackslash{}u00f0\textbackslash{}u0141\textbackslash{}u0128\textbackslash{}u0134} & 190 & \texttt{\textbackslash{}u00f0\textbackslash{}u0141\textbackslash{}u0127\textbackslash{}u00b1} & 191 & \texttt{\textbackslash{}u00ef\textbackslash{}u00ae\textbackslash{}u0131} \\
192 & \texttt{\textbackslash{}u00ed\textbackslash{}u0137\textbackslash{}u00ae} & 193 & \texttt{\textbackslash{}u00ed\textbackslash{}u012c\textbackslash{}u0143} & 194 & \texttt{\textbackslash{}u00ec\textbackslash{}u00a5\textbackslash{}u012b} & 195 & \texttt{\textbackslash{}u00ec\textbackslash{}u0142\textbackslash{}u00b0} \\
196 & \texttt{\textbackslash{}u00ec\textbackslash{}u0141\textbackslash{}u013b} & 197 & \texttt{\textbackslash{}u00ec\textbackslash{}u013f\textbackslash{}u00bf} & 198 & \texttt{\textbackslash{}u00ec\textbackslash{}u013f\textbackslash{}u00a9} & 199 & \texttt{\textbackslash{}u00ec\textbackslash{}u0139\textbackslash{}u00a4} \\
200 & \texttt{\textbackslash{}u00ec\textbackslash{}u0131\textbackslash{}u00b1} & 201 & \texttt{\textbackslash{}u00ec\textbackslash{}u012d\textbackslash{}u00b2} & 202 & \texttt{\textbackslash{}u00ec\textbackslash{}u012b\textbackslash{}u00a1} & 203 & \texttt{\textbackslash{}u00ec\textbackslash{}u0126\textbackslash{}u0132} \\
204 & \texttt{\textbackslash{}u00eb\textbackslash{}u00bc\textbackslash{}u013f} & 205 & \texttt{\textbackslash{}u00eb\textbackslash{}u00bb\textbackslash{}u0127} & 206 & \texttt{\textbackslash{}u00eb\textbackslash{}u00af\textbackslash{}u0133} & 207 & \texttt{\textbackslash{}u00eb\textbackslash{}u00a1\textbackslash{}u0133} \\
208 & \texttt{\textbackslash{}u00eb\textbackslash{}u0139\textbackslash{}u012f} & 209 & \texttt{\textbackslash{}u00eb\textbackslash{}u0136\textbackslash{}u012b} & 210 & \texttt{\textbackslash{}u00ea\textbackslash{}u00b8\textbackslash{}u0133} & 211 & \texttt{\textbackslash{}u00ea\textbackslash{}u013b\textbackslash{}u012d} \\
212 & \texttt{\textbackslash{}u00e3\textbackslash{}u00b3\textbackslash{}u00ac} & 213 & \texttt{\textbackslash{}u00e2\textbackslash{}u013d\textbackslash{}u00a4} & 214 & \texttt{\textbackslash{}u00e2\textbackslash{}u013c\textbackslash{}u00a7} & 215 & \texttt{\textbackslash{}u00e2\textbackslash{}u0126\textbackslash{}u00ac} \\
216 & \texttt{\textbackslash{}u00e1\textbackslash{}u00bd\textbackslash{}u013f} & 217 & \texttt{\textbackslash{}u00e1\textbackslash{}u00bc\textbackslash{}u00ae} & 218 & \texttt{\textbackslash{}u00e1\textbackslash{}u00ba\textbackslash{}u0122} & 219 & \texttt{\textbackslash{}u00e1\textbackslash{}u00b8\textbackslash{}u00b0} \\
220 & \texttt{\textbackslash{}u00e1\textbackslash{}u00a1\textbackslash{}u012e} & 221 & \texttt{\textbackslash{}u00da\textbackslash{}u0130} & 222 & \texttt{\textbackslash{}u00d1\textbackslash{}u00a8} & 223 & \texttt{\textbackslash{}u00f0\textbackslash{}u0141\textbackslash{}u0139\textbackslash{}u0123} \\
224 & \texttt{\textbackslash{}u00f0\textbackslash{}u0141\textbackslash{}u0138\textbackslash{}u00b6} & 225 & \texttt{\textbackslash{}u00f0\textbackslash{}u0141\textbackslash{}u0138\textbackslash{}u0133} & 226 & \texttt{\textbackslash{}u00f0\textbackslash{}u0141\textbackslash{}u0138\textbackslash{}u0129} & 227 & \texttt{\textbackslash{}u00f0\textbackslash{}u0141\textbackslash{}u0137\textbackslash{}u00b3} \\
228 & \texttt{\textbackslash{}u00f0\textbackslash{}u0141\textbackslash{}u0137\textbackslash{}u00a2} & 229 & \texttt{\textbackslash{}u00f0\textbackslash{}u0141\textbackslash{}u0137\textbackslash{}u0142} & 230 & \texttt{\textbackslash{}u00f0\textbackslash{}u0141\textbackslash{}u0137\textbackslash{}u0140} & 231 & \texttt{\textbackslash{}u00f0\textbackslash{}u0141\textbackslash{}u0137\textbackslash{}u013f} \\
232 & \texttt{\textbackslash{}u00f0\textbackslash{}u0141\textbackslash{}u0137\textbackslash{}u013e} & 233 & \texttt{\textbackslash{}u00f0\textbackslash{}u0141\textbackslash{}u0137\textbackslash{}u013c} & 234 & \texttt{\textbackslash{}u00f0\textbackslash{}u0141\textbackslash{}u0137\textbackslash{}u0138} & 235 & \texttt{\textbackslash{}u00f0\textbackslash{}u0141\textbackslash{}u0136\textbackslash{}u00a9} \\
236 & \texttt{\textbackslash{}u00f0\textbackslash{}u0141\textbackslash{}u0136\textbackslash{}u00a4} & 237 & \texttt{\textbackslash{}u00f0\textbackslash{}u0141\textbackslash{}u0136\textbackslash{}u00a2} & 238 & \texttt{\textbackslash{}u00f0\textbackslash{}u0141\textbackslash{}u0136\textbackslash{}u0135} & 239 & \texttt{\textbackslash{}u00f0\textbackslash{}u0141\textbackslash{}u0136\textbackslash{}u0129} \\
240 & \texttt{\textbackslash{}u00f0\textbackslash{}u0141\textbackslash{}u0136\textbackslash{}u0125} & 241 & \texttt{\textbackslash{}u00f0\textbackslash{}u0141\textbackslash{}u0136\textbackslash{}u0124} & 242 & \texttt{\textbackslash{}u00f0\textbackslash{}u0141\textbackslash{}u0136\textbackslash{}u0122} & 243 & \texttt{\textbackslash{}u00f0\textbackslash{}u0141\textbackslash{}u0135\textbackslash{}u00bc} \\
244 & \texttt{\textbackslash{}u00f0\textbackslash{}u0141\textbackslash{}u0135\textbackslash{}u00aa} & 245 & \texttt{\textbackslash{}u00f0\textbackslash{}u0141\textbackslash{}u0135\textbackslash{}u0141} & 246 & \texttt{\textbackslash{}u00f0\textbackslash{}u0141\textbackslash{}u0134\textbackslash{}u00ba} & 247 & \texttt{\textbackslash{}u00f0\textbackslash{}u0141\textbackslash{}u0134\textbackslash{}u00b9} \\
248 & \texttt{\textbackslash{}u00f0\textbackslash{}u0141\textbackslash{}u0133\textbackslash{}u013f} & 249 & \texttt{\textbackslash{}u00f0\textbackslash{}u0141\textbackslash{}u0132\textbackslash{}u0122} & 250 & \texttt{\textbackslash{}u00f0\textbackslash{}u0141\textbackslash{}u0131\textbackslash{}u00af} & 251 & \texttt{\textbackslash{}u00f0\textbackslash{}u0141\textbackslash{}u0131\textbackslash{}u00a9} \\
252 & \texttt{\textbackslash{}u00f0\textbackslash{}u0141\textbackslash{}u0131\textbackslash{}u0134} & 253 & \texttt{\textbackslash{}u00f0\textbackslash{}u0141\textbackslash{}u0131\textbackslash{}u0131} & 254 & \texttt{\textbackslash{}u00f0\textbackslash{}u0141\textbackslash{}u0130\textbackslash{}u00bf} & 255 & \texttt{\textbackslash{}u00f0\textbackslash{}u0141\textbackslash{}u0130\textbackslash{}u0133} \\
\addlinespace[4pt]  
\bottomrule
\end{tabular}
\end{table*}
