# Supplementary material for: MolmoAct2: Action Reasoning Models for Real-world Deployment
Source: arXiv:2605.02881 source file (2026-05-08)
Supplement: Supplementary file 6 [file hyperparams_real_ablation_molmoact.tex]

\begin{table}[!htbp]
\centering
\footnotesize
\setlength\tabcolsep{4pt}

\begin{tabular}{l*{3}{>{\centering\arraybackslash}p{2.8cm}}}
\toprule
\multicolumn{1}{c}{} &
\multicolumn{3}{c}{\cellcolor{olive!5}\textbf{Task Name}} \\[-0.2em]
\cmidrule(lr){2-4}
\textbf{Parameter} & \texttt{close\_lip} & \texttt{rotate\_pot} & \texttt{pour\_tea} \\
\midrule
% Learning Rate      & \multicolumn{3}{c}{5e-4} \\
Steps              & 8K & 6K & 15K \\
Global Batch Size  & \multicolumn{3}{c}{64} \\
GPUs (H100s)       & \multicolumn{3}{c}{32} \\
Time (Hours)       & 4 & 3 & 8 \\
GPU Hours          & 128 & 96 & 256 \\
Multi-task Training     & \multicolumn{3}{c}{No} \\
Input Images            & \multicolumn{3}{c}{1 Third-person + 1 Wrist-mounted} \\
Image Size              & \multicolumn{3}{c}{640$\times$320 px (Resized to 320$\times$240 px)} \\
DoF                     & \multicolumn{3}{c}{7 (3 Translations + 3 Rotations + 1 Gripper State)} \\
Observation History     & \multicolumn{3}{c}{No (Single-step Inputs)} \\
Use Proprioception & \multicolumn{3}{c}{No} \\
Action Chunk Size       & \multicolumn{3}{c}{8 Steps (Naive Action Chunking with Close-loop Prediction)} \\
% LoRA Rank               & \multicolumn{3}{c}{32} \\
% LoRA Alpha              & \multicolumn{3}{c}{16} \\
% LoRA Dropout            & \multicolumn{3}{c}{0} \\
% LoRA Bias               & \multicolumn{3}{c}{None} \\
\# Trainable Params     & \multicolumn{3}{c}{97M LoRA adapter} \\
Image Augmentations     &
\multicolumn{3}{c}{%
  \parbox[t]{8.4cm}{\raggedright
\texttt{import torchvision.transforms as T}\\
\texttt{transform = T.Compose([}\\
\texttt{\hspace*{1em}T.RandomResizedCrop(size=(height, width), scale=(0.9, 0.9), ratio=(width/height, width/height)),}\\
\texttt{\hspace*{1em}T.Resize((height, width)),}\\
\texttt{\hspace*{1em}T.ColorJitter(}\\
\texttt{\hspace*{2em}brightness=0.2,}\\
\texttt{\hspace*{2em}contrast=(0.8, 1.2),}\\
\texttt{\hspace*{2em}saturation=(0.8, 1.2),}\\
\texttt{\hspace*{2em}hue=0.05}\\
\texttt{\hspace*{1em}),}\\
\texttt{])}
}} \\
\addlinespace[4pt]  
\bottomrule
\end{tabular}
\caption{\textbf{\molmoact's Post-training Hyperparameters for Evaluation on \molmoactdata.} We specify the hyperparameters for \molmoact post-training. Note that we conduct all our post-training experiments on \molmoactd, with a fixed learning rate of 5e-4, LoRA rank of 32, LoRA alpha of 16, LoRA dropout of 0, and no LoRA bias.}
\label{tab:hyperparams_real_ablation}
\end{table}
